# Supplementary material for: Graph-Guided Selective Unlearning for Language Models: Controlling Support Routes Beyond Forget Seeds
Source: arXiv:2608.26743 source file (2026-08-27)
Supplement: Supplementary file 3 [file operational_details.tex]

% Operational appendix for inclusion from main.tex.
% Required in the main preamble:
%   \newcolumntype{L}{>{\raggedright\arraybackslash}X}
% This file assumes that \method, tab:settings, and the appendix mode
% are already defined in main.tex. It intentionally contains no
% \documentclass, package imports, \appendix, \section, or \end{document}.

\subsection{Measurement methodology and operational phases}

We distinguish three phases. \emph{(i) Offline, corpus-level, reusable:} fact extraction,
support-graph construction, and optional GradAlign preprocessing, computed once per corpus and
cached. \emph{(ii) Per deletion request:} request grounding, one- and two-hop support-closure
retrieval, support scoring, actionability/retain-safety filtering, and the model update.
\emph{(iii) Offline validation:} lightweight checkpoint evaluation (development-time) and the full
adversarial route audit. ``Cost'' is wall-clock time unless noted. Only fact extraction issues
external GPT-4.1 calls; all other generations are local. All timings use GPT-2-medium on TOFU on a
single NVIDIA RTX 3090 at seed~42, so the results characterise one consistent, controlled
configuration.

\subsection{Full stage-level decomposition}

\begin{table}[htbp]
\centering
\caption{Full operational cost decomposition. The non-evaluation residual is observed wall time
minus logged evaluation time; it bundles model update, setup, and checkpointing and is not a
training-time measurement.}
\label{tab:cost-full}
\small
\begin{tabularx}{\textwidth}{@{}L L c c@{}}
\toprule
\textbf{Component} & \textbf{Measured time / scale} & \textbf{Ext.\ calls} & \textbf{Per req.?} \\
\midrule
Fact extraction & 4{,}005 QA $\rightarrow$ 11{,}786 triples (runtime not instrumented) & $\approx$4{,}005 nominal & No \\
Global graph construction & 4{,}005 nodes; 45{,}683 edges (runtime not instrumented) & 0 & No \\
Optional GradAlign preprocessing & 62.99\,s / 1{,}900 samples ($\approx$30.2/s) & 0 & No \\
Request-conditioned graph targeting & 11.4--33.4\,s (cache-hit) & 0 & \textbf{Yes} \\
Observed non-evaluation residual & $\approx$5.7--6.9\,min & 0 & Yes \\
Lightweight checkpoint evaluation & 5.1--6.6\,min & 0 & Dev-time \\
Full adversarial route audit & 63.0--83.1\,min; 4{,}464--5{,}376 local gen. & 0 & No \\
\bottomrule
\end{tabularx}
\end{table}

With cached artefacts, request-conditioned targeting required 11.4\,s (partial deletion), 33.0\,s
(entity and instance), and 33.4\,s (complete), averaging 25.9\,s. A matched Seed-Only runtime log was
not available, so Seed-Only is omitted from the operational comparison. For completeness---these are
full end-to-end workflow times under differing audit schedules, not a controlled speed comparison---raw
observed wall times were 5.85, 7.63, and 7.70\,h for \method{} and 5.49, 6.90, and 7.03\,h for DPO, on
complete, entity, and partial deletion respectively.

\subsection{Graph scale and sparsification}

\begin{table}[htbp]
\centering
\caption{Original graph versus the final sparse (mutual-kNN) graph with partial GradAlign
augmentation, on the 4{,}005-node TOFU corpus.}
\label{tab:scale}
\small
\begin{tabular}{@{}p{4.6cm}ccc@{}}
\toprule
\textbf{Metric} & \textbf{Original} & \textbf{Final} & \textbf{Change} \\
\midrule
Nodes & 4{,}005 & 4{,}005 & 0 \\
Undirected edges & 52{,}816 & 45{,}683 & $-13.51\%$ \\
Average degree & 26.38 & 22.81 & $-13.51\%$ \\
95th-percentile degree & 42 & 30 & $-28.57\%$ \\
Maximum degree & 112 & 30 & $-73.21\%$ \\
Density & 0.659\% & 0.570\% & lower \\
Connected components & 1 & 1 & 0 \\
Isolated nodes & 0 & 0 & 0 \\
\bottomrule
\end{tabular}
\end{table}

The extracted facts (11{,}786 triples; 1{,}805 unique heads, 1{,}189 relations, 5{,}756 tails) and
the final graph are persisted and loaded at request time rather than reconstructed, amortising
construction cost across requests. The edge file and a representative GradAlign cache occupy
approximately 7.81\,MB; extracted facts and other metadata are persisted separately. These results
are structural scalability indicators at one corpus size and do not constitute a multi-corpus-size
scaling benchmark.

\textbf{Maintainability (cache validity).} As a deployment requirement, cached facts, embeddings,
graph edges, and GradAlign signatures should be versioned against the corpus snapshot, extraction
model, embedding model, and graph configuration; a corpus or model update requires rebuilding the
affected artefacts before subsequent deletion requests.

\subsection{GradAlign characterisation and provenance}
\label{sec:grad}

GradAlign is a \emph{representation-gradient alignment proxy}: it computes the gradient of the
answer-token cross-entropy with respect to the final-layer hidden representation, L2-normalises it
per sample, and scores edges by clipped cosine similarity. It is not full parameter-gradient
similarity. GradAlign is an \emph{optional} component and is not claimed as an independent empirical
contribution.

\begin{table}[htp]
\centering
\caption{GradAlign cache and edge statistics for the representative artefact (GPT-2-medium,
1{,}024-dimensional representations).}
\label{tab:gradalign}
\small
\begin{tabular}{@{}p{7.1cm}c@{}}
\toprule
\textbf{Metric} & \textbf{Value} \\
\midrule
Cached signatures (1{,}024-dim float16; 0 unusable) & 1{,}991 \\
Cache size & 4.07\,MB \\
Edges with both endpoint signatures & 17{,}108 (37.45\%) \\
Edges with non-zero GradAlign & 16{,}102 (35.25\%) \\
Mean / median GradAlign (affected edges) & 0.301 / 0.264 \\
90th / 95th percentile (affected edges) & 0.596 / 0.702 \\
Mean GradAlign share of combined weight (affected edges) & 21.12\% \\
\bottomrule
\end{tabular}
\end{table}

On the edges where it is defined, GradAlign contributes approximately one-fifth of the combined edge
weight on average (its contribution depends on the fixed coefficient $\lambda=0.7$). The
representative cache was constructed around the \emph{complete}-deletion seed neighbourhood
(1{,}991 signatures), giving full coverage for complete deletion (100\%) and partial coverage for the
partial (45.2\%) and entity/instance (83.5\%) settings; edges outside the cached subset receive a
GradAlign score of zero. GradAlign is an optional component, and we report these statistics only to
characterise the signal: we \textbf{make no cross-task GradAlign effectiveness claim}, which would
require uniform per-task caches.

% \subsection{Reliability controls}

% \begin{itemize}
% \item \textbf{Frozen evaluation manifests}: fixed sample and route sets, recorded for all three tasks.
% \item \textbf{Deterministic environment}: seed 42 and hardware metadata recorded; local-files-only model loading prevents version drift.
% \item \textbf{Bounded support expansion}: mutual-kNN ($K_{\mathrm{edge}}=30$), 1-/2-hop closure, top-$k$ caps, personalised PageRank with bounded top-60/min-15 support, and a fixed 64-item retain frontier; selected support sets contained 46--145 neighbours.
% \item \textbf{Staged graph activation}: a seed-only warm-up precedes graph-enabled steps (see the core implementation settings, Table~\ref{tab:settings}). A measured benefit is not claimed; an ablation is needed.
% \item \textbf{Actionability and retain-safety gates}: ambiguous neighbours are excluded rather than auto-forgotten or auto-retained.
% \item \textbf{Automated edge-integrity audit}: 0 self-loops, 0 duplicate edges, 0 non-finite values, 0 out-of-range components, 0 weight-formula mismatches.
% \item \textbf{Rule-based adversarial route prompts}: direct, paraphrase, indirect, cloze, related-fact, list-summary, relation-inversion, and entity-alias routes generated offline, incurring no external-LLM cost.
% \end{itemize}

\subsection{Evaluation-cost optimization}

In the recorded RTX 3090 runs, logged evaluation accounted for 98.0--98.8\% of observed wall time,
confirming that evaluation cadence---not support selection---dominates \method{}'s runtime. A hybrid
schedule (frequent lightweight evaluation; full route audit at selected milestones) used 26{,}880
adversarial generations and 7.70\,h on partial deletion, versus 79{,}200 generations and 16.73\,h
under a full-audit schedule---66.1\% fewer generations and 54.0\% lower wall time. Because the two
runs were not otherwise identical, this is evidence that \emph{audit cadence is a major operational
cost lever}, not a controlled algorithmic speedup.

\subsection{Measurement scope}

\begin{itemize}
\item The model-update figure is an observed non-evaluation residual (wall time minus logged evaluation), not a pure training-time measurement.
\item GradAlign is optional and its representative cache covers the complete-deletion neighbourhood (\S\ref{sec:grad}); we therefore make no cross-task GradAlign effectiveness claim.
\item Per-generation audit cost is observed throughput, not normalised for generated length or batching.
\item The reliability evidence concerns reproducibility, artefact integrity, bounded execution, and evaluation consistency; it does not constitute a statistical variance analysis across random seeds (all results use a single seed).
\end{itemize}
